# Supplementary material for: Generative AI Misuse: A Taxonomy of Tactics and Insights from Real-World Data
Source: arXiv:2406.13843 source file (2024-06-21)
Supplement: Supplementary file 1 [file table_appendix_strategies.pdf]

| Goal | Strategy | Use of GenAI | Tactic |
|---|---|---|---|
| Scam & Fraud | Celebrity scam ads | Impersonate celebrities or public figures to promote fraudulent investment scams | Impersonation |
| | Forgery | Forge documents to bypass identity verification | Falsification |
| | | Generate media (songs or books) that appear to have been created by known artists and sell them as authentic | Appropriateness Likeness + Counterfeit |
| | Phishing scam | Generate content to run targeted phishing scams at scale (e.g. business email compromise (BEC) campaigns.) | Scale & Amplification + Targeting/Personalization |
| | | Mimic an organisation's trademark to increase legitimacy of phishing. | Targeting/Personalization + Counterfeit |
| | | Create fake personas to carry out romance scams at scale | Sockpuppeting + Scale & Amplification |
| | | Impersonate a trusted individual (a loved one in distress, or a senior colleague) to steal funds | Impersonation |
| | Sextortion | Generate NCII of individuals from public social media photos to run sextortion schemes. | NCII + Scale & Amplification |
| | | Impersonate authorities to blackmail individuals | Impersonation |
| | Information theft | Impersonate public figures to access privileged information. | Impersonation |
| | Malware | Create copycat websites to trick users into downloading malware. | Counterfeit |
| | | Create fake tutorial videos to influence individuals to download stealer malware. | Sockpuppeting |

| | | | |
|---|---|---|---|
| **Opinion Manipulation** | Astroturfing | Create the impression of widespread grassroots support for or opposition against a cause | Sockpuppeting + Scale & Amplification |
| | | Create the impression of popular approval of a product (covert/spammy advertising) at scale | Scale & Amplification + Sockpuppeting |
| | Defamation | Alter appearance of politicians to make them look older | Appropriated Likeness |
| | | Impersonate politicians or political dissidents making abusive statements | Impersonation |
| | | Generate media of politicians in compromising situation | Appropriated Likeness |
| | Digital resurrection | Impersonate deceased victims to plead for a cause (e.g. gun reform) | Impersonation |
| | Disinformation | Impersonate politicians falsely endorsing specific political positions or claiming electoral victory | Impersonation |
| | | Generate false images of emotionally charged and politically divisive issues. | Falsification |
| | | Alter the likeness of dissidents or protesters | Appropriated Likeness |
| | | Generate images or stories of fake crisis events | Falsification |
| | Political outreach | Create personalised campaign robocallers on behalf of candidates. | Sockpuppeting + Targeting & Personalization |
| | | Generate robocalls to conduct outreach to voters in their language. | Appropriated Likeness |
| | Image cultivation | Generate media that create a positive impression of a public figure. | Appropriated Likeness + Falsification |
| | Voter suppression | Impersonate politician giving misleading election information | Impersonation |
| | News hijacking | Interrupt news broadcasts to air AI-generated media. | Sockpuppeting + Falsification |

| | | | |
|---|---|---|---|
| **Monetization & Profit** | Botnet | Operate botnets to perform revenue-generating actions | Sockpuppeting + Scale & Amplification |
| | Content farming | Generate high volumes of fake clickbait articles to optimise ad revenue | Falsification + Scale & Amplification |
| | | Mimic or recycle existing original content at scale by adding text and voiceovers. | IP Infringement + Scale & Amplification |
| | Deepfake commodification | Generate sexually explicit deepfakes of celebrities for sale | NCII |
| | | Create and sell chatbot impersonating politicians to answer election-related questions | Impersonation |
| | Plagiarism | Plagiarise original content across media for monetisation | IP Infringement |
| | Shirking | Generate fake documentation (e.g. legal filings) to automate one's labour. | Falsification |
| | | Create fake personas to produce product reviews. | Sockpuppeting |
| | Undressing services | Generate NCII of individuals as a paid service. | NCII |
| **Cyberattacks** | Target identification | Automate research and identification of high-value organisational targets and their vulnerabilities. | Scale & Amplification |
| | Resource development | Coding assistance for operation and automation of cyberattack-related tasks (e.g. targeted malware development) | Scale & Amplification + Targeting & Personalization |
| **Harassment** | Bullying | Generate NCII of private individuals or public figures (e.g. journalists) to bully or silence them. | NCII + CSAM |
| | Defamation | Generate audio and video clips of celebrities and private individuals making abusive or racist statements | Impersonation |
| | Doxxing | Generate audio clips of content creators reading aloud their own address. | Appropriated Likeness |
| **Reach** | Plagiarism | Plagiarise competitors' website content to maximise reach. | IP Infringement |
| | Digital resurrection | Create fake videos of deceased individuals narrating the events of their death. | Sockpuppeting |
| | Content farming | Generate bogus news articles at scale to boost website in search results. | Falsification + Scale & Amplification |
| **Subversion** | Anti-scraping | Poisoning training data to prevent copyrighted data scraping | Poisoning |
